# Supplementary material for: TroVE: Inducing Verifiable and Efficient Toolboxes for Solving Programmatic Tasks
Source: arXiv:2401.12869 source file (2024-01-23)
Supplement: Supplementary file 1 [file d_optimal-ordering.tex]

\section{Exploring Optimal Ordering}
\label{app:d:optimal-ordering}

We have shown that \textsc{TroVE} is robust to randomized ordering. We further investigate if a potentially optimal ordering exists that yields the best performance.

We hypothesize that an optimal ordering clusters examples using the same function. To get example clustering information, we take the results from running \textsc{TroVE}, and group together examples that use the same function in their solutions. We rank function clusters from the highest usage frequency to the lowest, to prioritize major function categories. We order examples in each cluster by their original order in the dataset. If an example uses multiple functions, we only include it in the last appearing function cluster, to ensure all functions required (should be) available. We denote this as \textit{post-hoc}.
\dfcomment{It's not too clear to me why this would be the optimal ordering. Is Trove more likely to use recently induced rather than older functions? If not, why is it helpful to have sequences of examples that all use the same function?}

\begin{table}[ht]
\small 
\centering 
\resizebox{0.45\textwidth}{!}{
    \begin{tabular}{l|r|r|r}
    \toprule
    \multirow{2}{*}{\textbf{Method}} & \multicolumn{3}{c}{\textbf{Evaluation Metrics}} \\
    {} & \multicolumn{1}{c|}{acc $\uparrow$} & \multicolumn{1}{c|}{\# ops $\downarrow$} & \multicolumn{1}{c}{\# lib $\downarrow$} \\
    \midrule
    \multicolumn{4}{c}{\hlcell MATH$_{algebra}$} \\
    \midrule
    {original} & {0.25} & {18.8} & {10} \\
    {post-hoc} & {0.26} & {19.0} & {10} \\
    \midrule
    \multicolumn{4}{c}{\hlcell HiTab} \\
    \midrule
    {original} & {0.18} & {9.3} & {5} \\
    {post-hoc} & {0.17} & {9.0} & {10} \\
    \midrule
    \multicolumn{4}{c}{\hlcell \textsc{GQA}} \\
    \midrule
    {original} & {0.43} & {20.6} & {6} \\
    {post-hoc} & {0.46} & {20.1} & {8} \\
    \bottomrule
    \end{tabular}
}
\vspace{-1mm}
\caption{\textsc{CodeLLaMa} results with post-hoc ordering.}
\vspace{-1mm}
\label{tab:optimal-ordering}
\end{table}

From \autoref{tab:optimal-ordering}, post-hoc example ordering slightly improves on three datasets, however, not comprehensively on all metrics. In MATH$_{algebra}$, accuracy increases by $+ 1\%$ but at the cost of $+ 0.2$ more operations. In Hitab, although accuracy drops by $- 2\%$, but it saves operation counts by $- 0.3$. In GQA, both accuracy ($+ 3\%$) and complexity ($- 0.5$) scores better, but at the cost of 2 more functions.
